# Supplementary material for: Making the best of a bad situation: a multiscale approach to free energy calculation
Source: arXiv:1901.04455 ancillary file (2019-02-22)
Supplement: Supplementary file 1 [file SupportingInformation.pdf]

# Supporting information for: Making the best of a bad situation: a multiscale approach to free energy calculation

Michele Invernizzi*,†,¶ and Michele Parrinello‡,¶

†*Department of Physics, ETH Zurich c/o USI Campus, Lugano, Switzerland*

‡*Department of Chemistry and Applied Biosciences, ETH Zurich c/o USI Campus, Lugano, Switzerland*

¶*Facoltà di Informatica, Instituto di Scienze Computationali, and National Center for Computational Design and Discovery of Novel Materials MARVEL, Università della Svizzera italiana (USI), Via Giuseppe Buffi 13, CH-6900 Lugano, Switzerland*

E-mail: michele.invernizzi@phys.chem.ethz.ch

## 1 Sampling with different CVs

We would like to give a simple example of the different sampling that can be accomplished by using different kind of collective variables for biasing. We use alanine dipeptide, and we run three different WTMetaD simulations ($\gamma = 10$) biasing respectively only the "bad" angle $\psi$, only the "good" angle $\phi$, and both angles. The three simulation require very different time to converge, with the bad angle one requiring more than one order of magnitude more time, but we show in Fig. S1 the same number of points for each simulation. We used WTMetaD in this example, but the point we want to make is not limited to this method, it is a characteristic shared with all CV-based enhanced sampling techniques. We would obtain

the same figure if we were to use a static bias instead: respectively $V(\psi) = -(1-1/\gamma)F(\psi)$, $V(\phi) = -(1-1/\gamma)F(\phi)$, and $V(\phi,\psi) = -(1-1/\gamma)F(\phi,\psi)$.

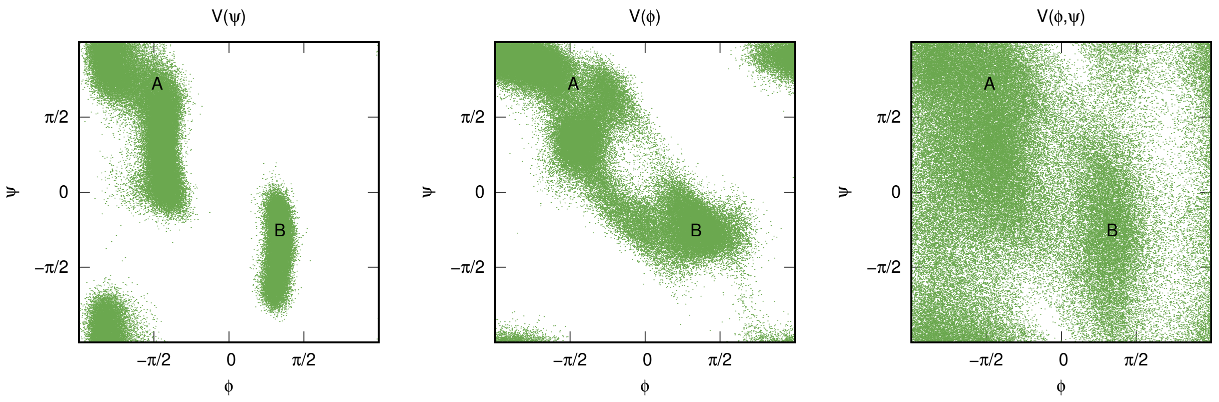


Figure S1: Different sampling obtained by employing different CVs for building the bias in WTMetaD. All simulations are fully at convergence, and only 100000 point are shown for each one. For a reference free energy see Fig. 5 of main text.

It can be seen how, when a slow degree of freedom is missing from the bias, a lot of simulation time is spent in the minima, instead of exploring new configurations, and some high free energy region are almost never visited. Despite this, the three simulations all provide the same estimate for $\Delta F$, when using Eq. (15) to calculate it from the reweighting. This is due to the fact that the contribution from these high free energy regions is extremely small and can be safely ignored. If instead one is interested not only in the free energy difference, but on the full FES along a specific CV, a good strategy would be to directly bias also such CV.

# 2 Notes on Eq. (12) and (11)

We first define $\mathbf{s}_A$ and $\mathbf{s}_B$ as the points where $F_A$ and $F_B$ respectively are minimum, thus $F_A(\mathbf{s}_A) = 0$ and $F_B(\mathbf{s}_B) = 0$. If $A$ is the most stable basin, we can then explicitly write $\Delta F_h = F(\mathbf{s}_B) - F(\mathbf{s}_A)$, where $F(\mathbf{s})$ is the global FES.

Eq. (12) and (11) of the main text are strictly true only in the limit of

$$F_A(\mathbf{s}_B) \to \infty \quad \text{and} \quad F_B(\mathbf{s}_A) \to \infty \,. \tag{S1}$$

Outside of this limit, Eq. (12) holds true if we substitute $\Delta F_h$ with another quantity, that we call $\Delta F'_h$. The exact relation between these quantities is the following:

$$\Delta F_h = \Delta F'_h - \frac{1}{\beta} \log \left[ \frac{1 + e^{-\beta(F_B(\mathbf{s}_A) - \Delta F'_h)}}{1 + e^{-\beta(F_A(\mathbf{s}_B) + \Delta F'_h)}} \right] \,. \tag{S2}$$

Also, if condition (S1) does not hold, we have

$$\min[F(\mathbf{s})] = F(\mathbf{s}_A) = -\frac{1}{\beta} \log \left[ 1 + e^{-\beta(F_B(\mathbf{s}_A) - \Delta F'_h)} \right] \,, \tag{S3}$$

which in general is non-zero. A similar correction can be found also for Eq. (11).

In VES$\Delta F$ we use approximate estimates for the local basins and condition (S1) cannot formally be fulfilled, but from a practical point of view this does not constitute a problem. In fact, the difference between $\Delta F'_h$ and $\Delta F_h$ is typically some order of magnitude smaller than the uncertainty of the free energy calculation. For the sodium and the model system examples, this discrepancy stays well below $10^{-5}\, k_B T$, while for alanine dipeptide, where the employed CV is quite bad at distinguishing the two basins, it stays below $0.1\, k_B T$.

It is important to remember that this approximation does not affect in any way the $\Delta F$ or $\Delta F_h$ calculated through the reweighting procedure (as in Fig. 7 of main text).

# 3 Optimization algorithm

The optimization algorithm used in the second step of VES$\Delta F$, is a novel combination of the optimization algorithm commonly used in VES[S1,S2] and AdaGrad[S3] stochastic gradient descent algorithm.

In the present paper we only consider the case of two basins, thus we deal with one optimization parameter $\Delta F$ (or $\Delta F_h$, depending on the chosen normalization). Here however we present a more general version of the optimization algorithm, using a multidimensional vector of parameters $\boldsymbol{\alpha}$.

Following Ref. S1, we write gradient and Hessian of the VES functional:

$$\frac{\partial\Omega(\boldsymbol{\alpha})}{\partial\alpha_i} = -\left\langle\frac{\partial V(\mathbf{s};\boldsymbol{\alpha})}{\partial\alpha_i}\right\rangle_{V(\boldsymbol{\alpha})} + \left\langle\frac{\partial V(\mathbf{s};\boldsymbol{\alpha})}{\partial\alpha_i}\right\rangle_{p}, \tag{S4}$$

$$\begin{aligned}\frac{\partial^2\Omega(\boldsymbol{\alpha})}{\partial\alpha_i\partial\alpha_j} =& \beta\left[\left\langle\frac{\partial V(\mathbf{s};\boldsymbol{\alpha})}{\partial\alpha_i}\frac{\partial V(\mathbf{s};\boldsymbol{\alpha})}{\partial\alpha_j}\right\rangle_{V(\boldsymbol{\alpha})} - \left\langle\frac{\partial V(\mathbf{s};\boldsymbol{\alpha})}{\partial\alpha_i}\right\rangle_{V(\boldsymbol{\alpha})}\left\langle\frac{\partial V(\mathbf{s};\boldsymbol{\alpha})}{\partial\alpha_j}\right\rangle_{V(\boldsymbol{\alpha})}\right] + \\ & - \left\langle\frac{\partial^2 V(\mathbf{s};\boldsymbol{\alpha})}{\partial\alpha_i\partial\alpha_j}\right\rangle_{V(\boldsymbol{\alpha})} + \left\langle\frac{\partial^2 V(\mathbf{s};\boldsymbol{\alpha})}{\partial\alpha_i\partial\alpha_j}\right\rangle_{p},\end{aligned} \tag{S5}$$

where the averages are calculated either in the biased ensemble $\langle\cdot\rangle_{V(\boldsymbol{\alpha})}$ (by running the molecular dynamics), or in the target $p(\mathbf{s})$ ensemble $\langle\cdot\rangle_p$ (by explicit integration on a grid).

We make use of a second set of auxiliary parameters for updating the main one. At each iteration $n$, we have some auxiliary instantaneous iterate $\boldsymbol{\alpha}^{(n)}$, while the actual parameters are obtained as their averages

$$\bar{\boldsymbol{\alpha}}^{(n)} = \frac{1}{n+1}\sum_{k=0}^{n}\boldsymbol{\alpha}^{(k)}. \tag{S6}$$

Gradient and Hessian are always evaluated using this set of averaged parameters.

We use the above gradient and Hessian, Eq. (S4) and (S5), to define an effective gradient $\mathbf{g}^{(n)}$:

$$g_i^{(n)} = \frac{\partial\Omega\left(\bar{\boldsymbol{\alpha}}^{(n)}\right)}{\partial\alpha_i} + \sum_j\frac{\partial^2\Omega\left(\bar{\boldsymbol{\alpha}}^{(n)}\right)}{\partial\alpha_i\partial\alpha_j}\left(\alpha_j^{(n)} - \bar{\alpha}_j^{(n)}\right). \tag{S7}$$

In the spirit of the AdaGrad algorithm, we then introduce an history dependent damping factor $\mathbf{d}^{(n)}$:

$$d_i^{(n)} = \sqrt{\left[d_i^{(n-1)}\right]^2 + \left[g_i^{(n)}\right]^2}. \tag{S8}$$

We can now write the update rule for the auxiliary parameters:

$$\alpha_i^{(n+1)} = \alpha_i^{(n)} - \frac{\mu}{d_i^{(n)}} g_i^{(n)} , \tag{S9}$$

where $\mu$ is a fixed optimization hyperparameter. The standard VES optimization algorithm is retrieved if we set $d_i^{(n)} = 1$ for each $i$ and $n$.

## 3.1 Hyperparameters choice

The hyperparameters the user needs to set in VES$\Delta F$ are essentially three:

- the bias factor for the target distribution, $\gamma$
- the update stride for the parameters, during which the ensemble averages are estimated
- the optimization step $\mu$

For the choice of the bias factor we use criteria similar to those employed for well-tempered VES[S4] and WTMetaD,[S5] the main difference being that our method is less sensitive to the choice of $\gamma$. In particular, contrary to what happens in WTMetaD, the value of $\gamma$ does not have a direct impact on the speed at which bias is added, allowing for more flexibility.

We chose an update stride of 1 ps that is a typical value for both MetaD and standard VES.

The choice of the optimization step $\mu$ is in our experience the most crucial, but it was not a hard one. We did not try systematically to optimize this choice, since there is a reasonable range of "good" values. We did notice, though, that an extreme choice of this hyperparamer can make convergence terribly slow. In the systems studied here, we noticed that the choice of $\mu$ had a direct impact on the speed at which the parameter $\alpha$ (thus $\Delta F$ or $\Delta F_h$) grows, independently of other factors like $\gamma$ and the number of multiple walkers. As an empirical rule at the beginning of the optimization, before any transition has taken place, we have

$\alpha(t) \approx 1.2\mu\sqrt{t}$. Further investigation is needed in order to provide a simple rule of thumb for the choice of $\mu$.

## 4 Illustrative model

To run the illustrative model considered in Sec. 3 of the main text we use a simple molecular dynamics code implemented in PLUMED[S6] (version 2.4 or higher), called `ves_md_linearexpansion`. We used the default parameters for the simulation (`tstep=0.005`, `temperature=1`, `friction=10`) and the Wolfe-Quapp potential,

$$U(x, y) = x^4 + y^4 - 2\,x^2 - 4\,y^2 + xy + 0.3\,x + 0.1\,y\,, \tag{S10}$$

which we rotated of an angle $\theta = -0.15\pi$ by rotating the coordinates, thus:

$$\begin{aligned} x &\to x\cos\theta - y\sin\theta \\ y &\to x\sin\theta + y\cos\theta \end{aligned} \tag{S11}$$

The resulting potential is:

$$\begin{aligned} U(x, y) =& 1.34549\,x^4 + 1.90211\,x^3y + 3.92705\,x^2y^2 \\ &- 6.44246\,x^2 - 1.90211\,xy^3 + 5.58721\,xy + 1.33481\,x \\ &+ 1.34549\,y^4 - 5.55754\,y^2 + 0.904586\,y + 18.5598\,, \end{aligned} \tag{S12}$$

where the last shift term is added just to put the minimum at zero.

For the MetaD simulations we always use the following parameters: `PACE=500`, `HEIGHT=1.2`, `SIGMA=0.35`, `BIASFACTOR=10`, and store the bias on a grid of `GRID_BIN=300`, `GRID_MIN=-3`, `GRID_MAX=3`. The local free energy basins obtained for VES$\Delta F$ are stored on the same kind of grid, and required a total combined number of $2.11 \times 10^6$ simulation steps. The parameters used for the VES optimization are: `AV_STRIDE=500`, `M_STEP=0.05`, `BIASFACTOR=10`.

# 5 Alanine dipeptide

For the Alanine dipeptide simulations we use GROMACS[S7] patched with PLUMED. The setup is the same of Ref. S1, namely: NVT simulation in a vacuum, Amber99-SB[S8] force field, time step 2 fs, temperature 300 K, velocity rescaling termostat.[S9]

The MetaD simulations use the following parameters: `PACE=500`, `HEIGHT=1.2`, `SIGMA=0.35`, `BIASFACTOR=10`, and store the bias on a grid of `GRID_BIN=100`, `GRID_MIN=-pi`, `GRID_MAX=pi`. For the TTMetaD the same parameters are used, plus `TTBIASFACTOR=10`, `TRANSITIONWELL0=0.8`, `TRANSITIONWELL1=2.7`. The local free energy basins obtained for VES$\Delta F$ are stored on the same kind of grid, and required a total combined simulation time of 7.10 ns. The parameters used for the VES optimization are: `AV_STRIDE=500`, `M_STEP=0.05`, `BIASFACTOR=10`.

## 5.1 Results

We show here more in detail some of the results from our alanine dipeptide simulations. We performed a set of calculations with different number of walkers, comparing WTMetaD, TTMetaD and VES$\Delta F$ methods. Each calculation is repeated 10 times to gauge the error. All replicas and walkers start from basin $A$ with different initial conditions and random seed. The same initial configurations are used for the three methods.

We notice how in this case TTMetaD converges better than WTMetaD. It can be seen how VES$\Delta F$ convergence is smoother than MetaD, and gains more from the reweighting procedure.

Finally, as noticed in the main text, increasing the number of walkers allows for a better sampling of the unbiased slow degree of freedom, and thus ameliorates convergence. This is typical of suboptimal CVs, whereas if an optimal CV is used one soon reaches a plateau in sampling efficiency when increasing the number of multiple walkers.

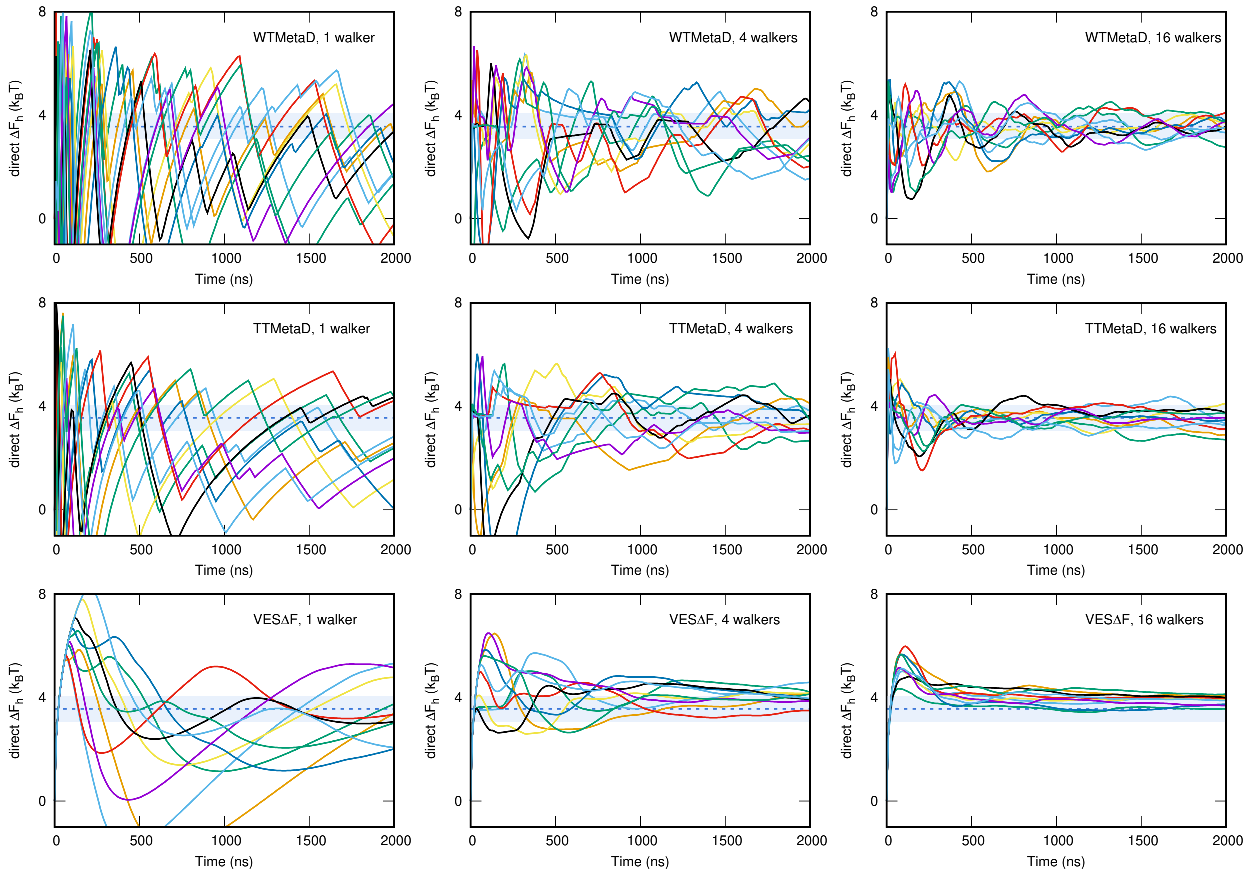


Figure S2: Comparison between alanine $\Delta F_h$ convergence for 10 replicas using WTMetaD, TTMetaD and VES$\Delta F$, with 1, 4 and 16 multiple walkers ($\gamma = 10$). The $\Delta F_h$ is estimated directly form the bias applied, via the relation $F(s) = -(1 - 1/\gamma)^{-1} V(s)$. The reference blue stripe is $1\, k_B T$ thick.

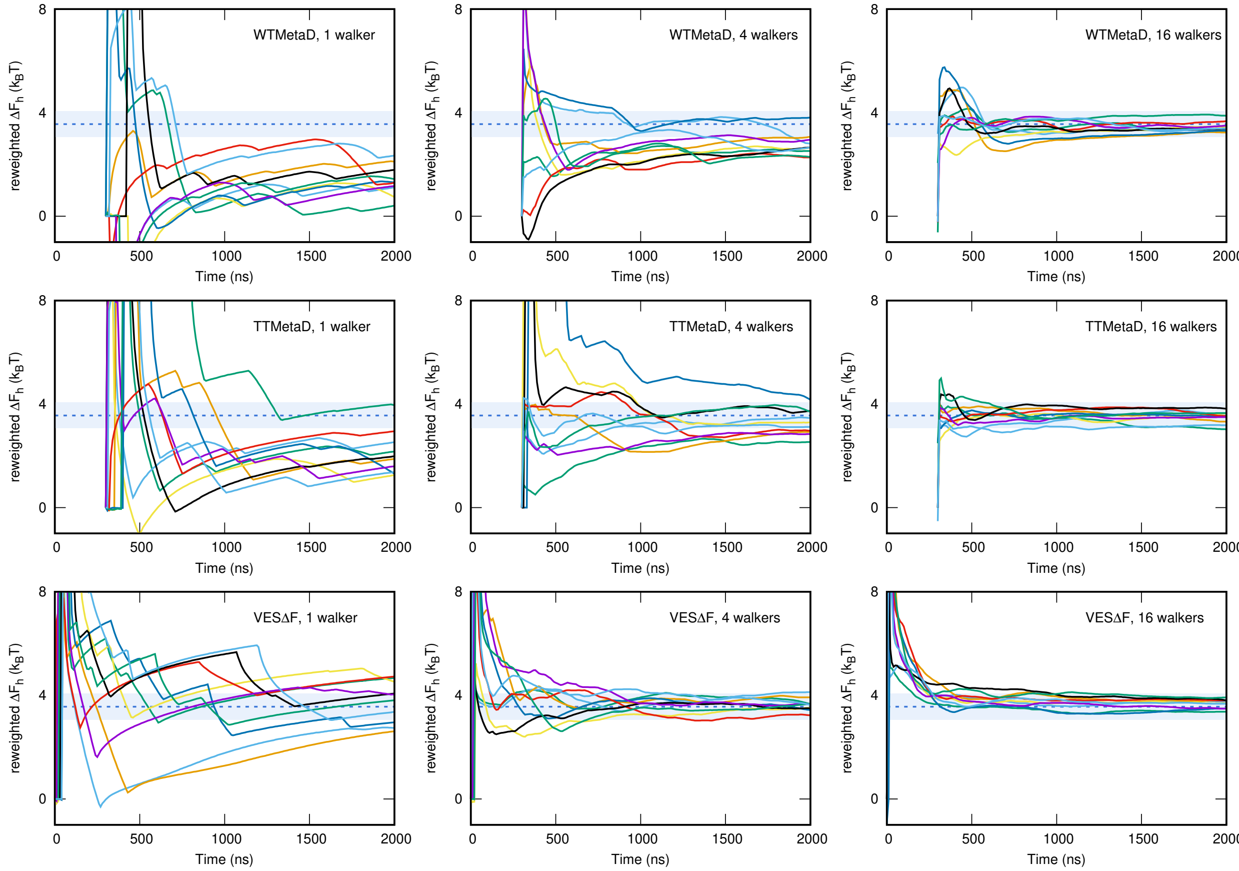


Figure S3: Comparison between alanine $\Delta F_h$ convergence for 10 replicas using WTMetaD, TTMetaD and VES$\Delta F$, with 1, 4 and 16 multiple walkers ($\gamma = 10$). The $\Delta F_h$ is estimated throug the reweighting procedure described in the main text. In the case of MetaD we must exclude from the reweighting an initial transient, in which the system is out of equilibrium and the estimate of $c(t)$ is unreliable. The reference blue stripe is $1\, k_B T$ thick.

# 6 Sodium

For the sodium simulations we use LAMMPS[S10] patched with PLUMED. An embedded atom model (EAM) is used as interatomic potential,[S11] molecular dynamics time step is 2 fs, and temperature 350 K. We use the stochastic velocity rescaling thermostat[S9] (0.1 ps relaxation time) and an isotropic Parrinello-Rahman barostat[S12] (1 ps relaxation time). The system size is 250 atoms.

The Debye structure factor CV we used is implemented in a development version of PLUMED, but it is openly available upon request and we plan to make it public in the near future. This collective variable is extensively described in Ref. S13. We consider the first structure factor peak of the bcc solid, at a scattering frequency $Q = 2.070595$ Å$^{-1}$ and with a cutoff $R_c = 10.5$ Å.

For the MetaD simulations we use the following parameters: `PACE=500`, `HEIGHT=10`, `SIGMA=0.2`, `BIASFACTOR=20`, and store the bias on a grid of `GRID_BIN=200`, `GRID_MIN=1`, `GRID_MAX=3`. The local free energy basins obtained for VES$\Delta F$ are stored on the same kind of grid, and required a total combined simulation time of 6.75 ns. The parameters used for the VES optimization are: `AV_STRIDE=500`, `M_STEP=1`, `BIASFACTOR=20`. In both cases we used 4 walkers, all initialized in different random configurations inside basin $A$, obtained from an unbiased run. The reference $\Delta F_h$ value was obtained from a longer WTMetaD 10 walkers run.

# References


(S1) Valsson, O.; Parrinello, M. Variational approach to enhanced sampling and free energy calculations. *Physical Review Letters* **2014**, *113*, 1–5.

(S2) Bach, F.; Moulines, E. Non-strongly-convex smooth stochastic approximation with convergence rate O(1/n). Advances in Neural Information Processing Systems 26. 2013; pp 773–781.

(S3) Duchi, J.; Hazan, E.; Singer, Y. Adaptive subgradient methods for online learning and stochastic optimization. The Journal of Machine Learning Research. 2011; pp 2121–2159.

(S4) Valsson, O.; Parrinello, M. Well-tempered variational approach to enhanced sampling. *Journal of Chemical Theory and Computation* **2015**, *11*, 1996–2002.

(S5) Barducci, A.; Bussi, G.; Parrinello, M. Well-Tempered Metadynamics: A Smoothly Converging and Tunable Free-Energy Method. *Physical Review Letters* **2008**, *100*, 020603.

(S6) Tribello, G. A.; Bonomi, M.; Branduardi, D.; Camilloni, C.; Bussi, G. PLUMED 2: New feathers for an old bird. *Computer Physics Communications* **2014**, *185*, 604–613.

(S7) Abraham, M. J.; Murtola, T.; Schulz, R.; Páll, S.; Smith, J. C.; Hess, B.; Lindahl, E. GROMACS: High performance molecular simulations through multi-level parallelism from laptops to supercomputers. *SoftwareX* **2015**, *1-2*, 19–25.

(S8) Hornak, V.; Abel, R.; Okur, A.; Strockbine, B.; Roitberg, A.; Simmerling, C. Comparison of multiple Amber force fields and development of improved protein backbone parameters. *Proteins: Structure, Function, and Bioinformatics* **2006**, *65*, 712–725.

(S9) Bussi, G.; Donadio, D.; Parrinello, M. Canonical sampling through velocity rescaling. *The Journal of Chemical Physics* **2007**, *126*, 014101.

(S10) Plimpton, S. Fast Parallel Algorithms for Short-Range Molecular Dynamics. *Journal of Computational Physics* **1995**, *117*, 1–19.

(S11) Wilson, S. R.; Gunawardana, K. G. S. H.; Mendelev, M. I. Solid-liquid interface free energies of pure bcc metals and B2 phases. *The Journal of Chemical Physics* **2015**, *142*, 134705.

(S12) Parrinello, M.; Rahman, A. Polymorphic transitions in single crystals: A new molecular dynamics method. *Journal of Applied Physics* **1981**, *52*, 7182–7190.

(S13) Niu, H.; Piaggi, P. M.; Invernizzi, M.; Parrinello, M. Molecular dynamics simulations of liquid silica crystallization. *Proceedings of the National Academy of Sciences* **2018**, *115*, 5348–5352.
